# Supplementary material for: Coastal Flood Risk in the Mortgage Market: Storm Surge Models' Predictions vs. Flood Insurance Maps
Source: arXiv:2006.02977 source file (2020-06-09)
Supplement: Supplementary file 1 [file appendix_census.tex]

\captionsetup[table]{labelformat=empty,skip=1pt}
\begin{longtable}{ll}
\toprule
table\_label & table\_code \\ 
\midrule
Median age & B01002\_001E \\ 
Median house value & B25077\_001E \\ 
Median monthly owner cost & B25088\_001E \\ 
Median monthly owner cost (with a mortgage) & B25088\_002E \\ 
Monthly owner cost as \% of income (with a mortgage) & B25092\_002E \\ 
With a mortgage & B25096\_002E \\ 
Total (for mortgage status) & B25096\_001E \\ 
Total number of households & B09005\_001E \\ 
Total population & B01003\_001E \\ 
Total population (for race) & B02001\_001E \\ 
White population & B02008\_001E \\ 
Black population & B02009\_001E \\ 
Hispanic population & B03001\_003E \\ 
Total population (for hispanic count) & B03001\_001E \\ 
Asian population & B02011\_001E \\ 
Median household income & B19013\_001E \\ 
Below poverty level & B17001\_002E \\ 
Total population (for poverty level) & B17001\_001E \\ 
Total population (for means of transportation) & B08006\_001E \\ 
Means of Transportation Car, truck, or van & B08006\_002E \\ 
Total population (for labor force and health insurance coverage) & B27011\_001E \\ 
Not in labor force!!no health insurance coverage & B27011\_017E \\ 
In labor force!!Employed!!No health insurance coverage & B27011\_007E \\ 
In labor force!!Unemployed!!No health insurance coverage & B27011\_012E \\ 
Median gross rent & B25031\_001E \\ 
Total (for tenure by units in structure) & B25032\_001E \\ 
Total!!Owner-occupied housing units & B25032\_002E \\ 
Total!!Owner-occupied housing units!!Mobile home & B25032\_011E \\ 
Total!!Owner-occupied housing units!!Boat, RV, van, etc. & B25032\_012E \\ 
Total!!Renter-occupied housing units & B25032\_013E \\ 
Total!!Renter-occupied housing units!!Mobile home & B25032\_022E \\ 
Total!!Renter-occupied housing units!!Boat, RV, van, etc. & B25032\_023E \\ 
\bottomrule
\end{longtable}
